# Supplementary material for: GOTCHA: Real-Time Video Deepfake Detection via Challenge-Response
Source: arXiv:2210.06186 source file (2024-05-23)
Supplement: Supplementary file 1 [file misc.tex]

% !TEX root = ../main.tex 

\begin{figure}[h!!]
\centering
\hspace{-1em}
    \subfloat[Seg. mask mismatch]{%
        \begin{minipage}{0.60\columnwidth}
            \includegraphics[width=0.5\columnwidth]{./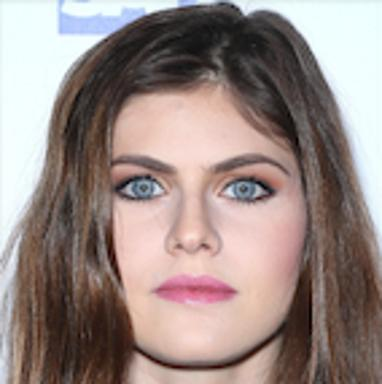}%
            \includegraphics[width=0.5\columnwidth]{./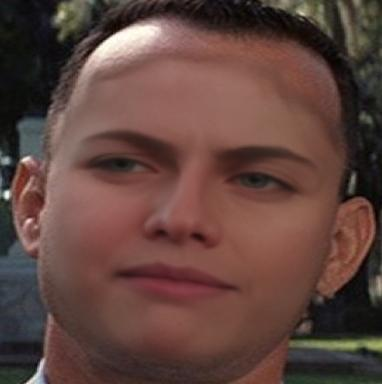}
        \end{minipage}
    }\hspace{-0.15em}%
    
    \subfloat[Smiley \& Deepfake]{%
        \begin{minipage}{0.60\columnwidth}
            \includegraphics[width=0.5\columnwidth]{./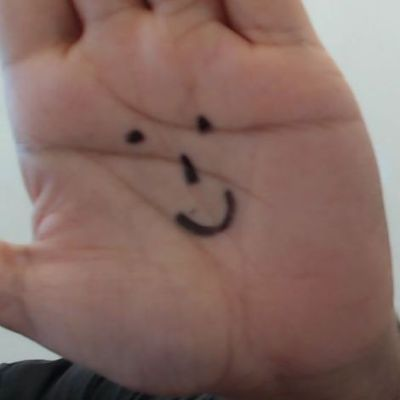}%
            \includegraphics[width=0.5\columnwidth]{./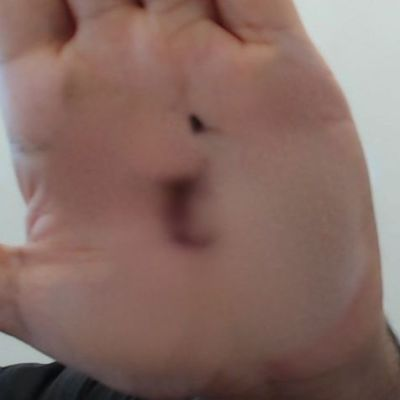}
        \end{minipage}
    }\hspace{-0.15em}%
    
    \subfloat[Fist \& deepfake on it]{%
        \begin{minipage}{0.60\columnwidth}
            \includegraphics[width=0.5\columnwidth]{./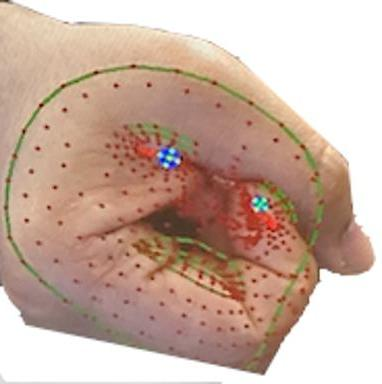}%
            \includegraphics[width=0.5\columnwidth]{./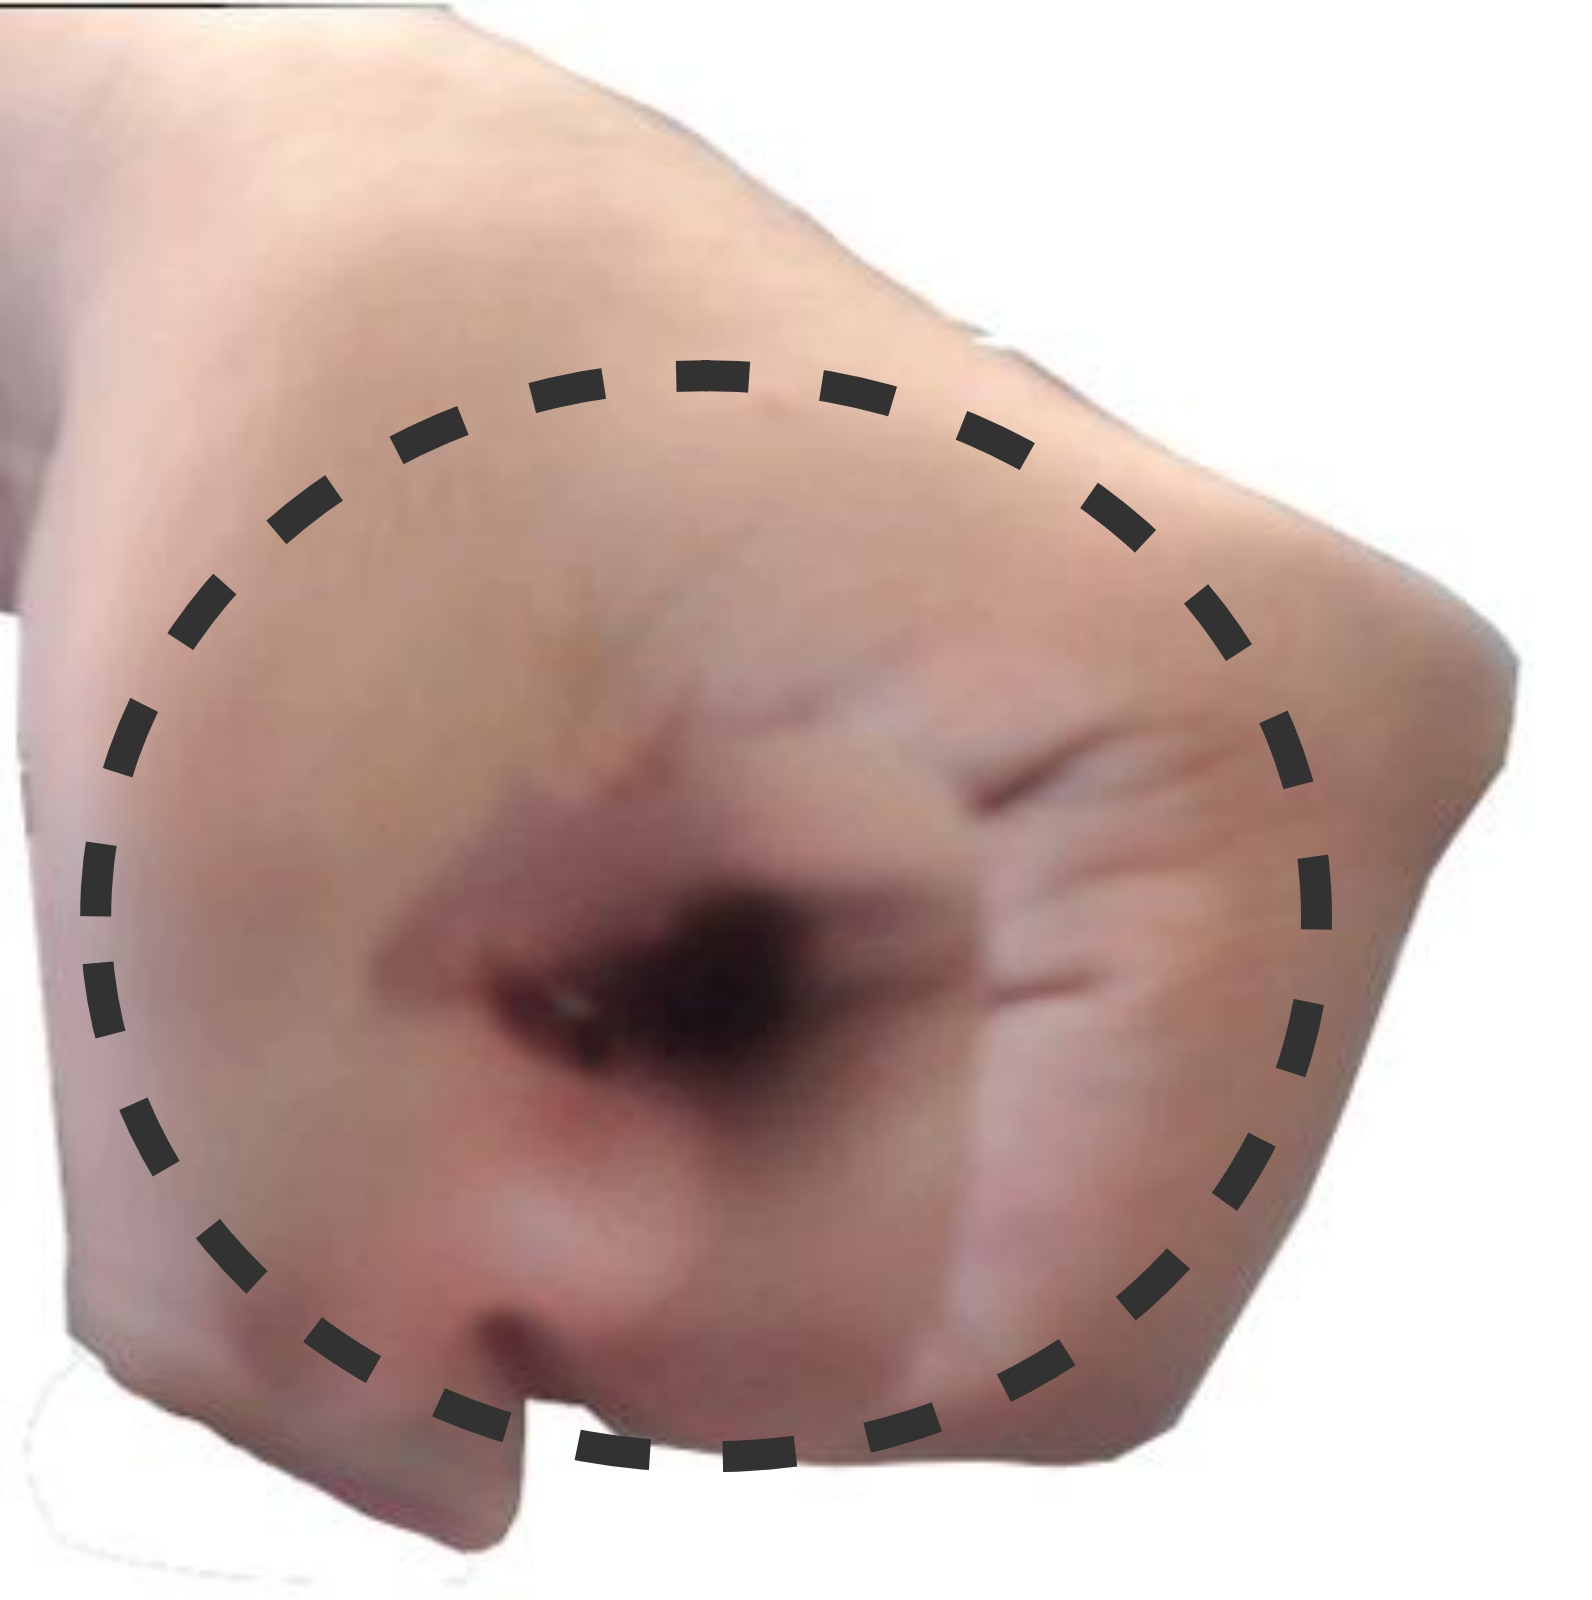}
        \end{minipage}
    }\hspace{-0.15em}%
    
    \subfloat[Misaligned by Occl.]{%
        \begin{minipage}{0.60\columnwidth}
            \includegraphics[width=0.5\columnwidth]{./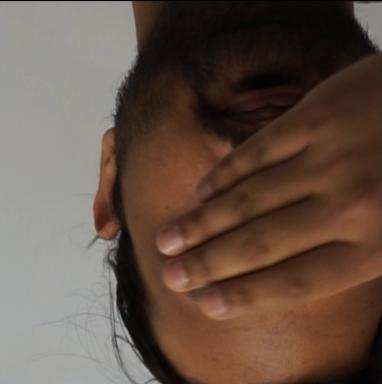}%
            \includegraphics[width=0.5\columnwidth]{./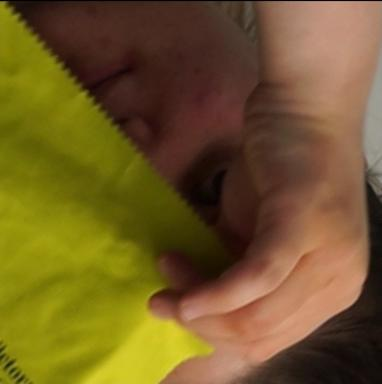}
        \end{minipage}
    }\hspace{-0.15em}%
    
    \subfloat[Face pack]{%
        \begin{minipage}{0.60\columnwidth}
            \includegraphics[width=0.5\columnwidth]{./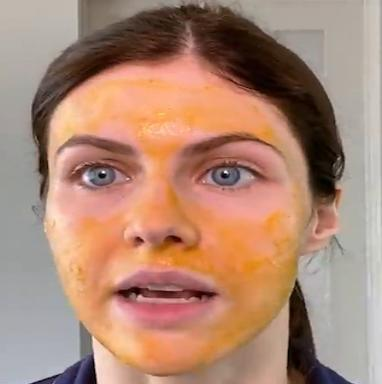}%
            \includegraphics[width=0.5\columnwidth]{./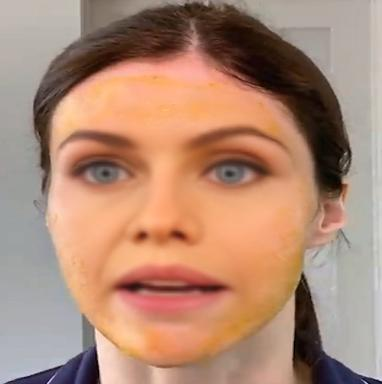}
        \end{minipage}
    }
\caption{This figure displays uncategorized samples exhibiting unexpected behaviors: (a) A discrepancy in the segmentation mask causes the source's hairline (left) to project onto the impersonator (right). (b)-(c) The face and landmarks are detected in these samples, leading to a corresponding deepfake (circled). (d) Occlusions create an inverted alignment. (e) A yellow face pack applied to the participant's face causes a color shift across the entire self-deepfake (where target identity equals imposter identity). Employing a self-deepfake eliminates the impact of skin color differences on the artifacts.}
\label{fig:misc}
\end{figure}
